# Supplementary material for: Towards Ubiquitous Intelligent Hand Interaction
Source: arXiv:2308.13543 source file (2023-08-21)
Supplement: Supplementary file 1 [file appendix.tex]

\section{Appendix}

% \begin{landscape}
\begin{table*}
  \vspace{-0.3cm}
  \centering
  \caption{The template scripts used by the experimenter to guide the user study tasks in four applications.}~\label{tab:task_description}
    \vspace{-0.3cm}
    \begin{tabularx}{\textwidth}{X|X|X|X}
    \toprule
    Application 1: Home Navigator & Application 2: Photo Album & Application 3: Whiteboard & Application 4: Text Editor \\
    \midrule
    \begin{enumerate}[1. , leftmargin=*, nosep]
        \item Move the cursor with index finger over a [APP Name] app icon.
        \item Tap with index finger on the [APP Name] app icon to launch the app.
        \item Swipe up with index finger and middle finger to return to the home.
        \item Swipe down with index finger and middle finger to return to the last opened app.
        \item Swipe left/right with index finger and middle finger to switch to the next/previous app.
        
    \end{enumerate} & 
    \begin{enumerate}[1. , leftmargin=*, nosep]
        \item Swipe left/right with index finger on trackpad to switch to the next/previous photo.
        \item Move thumb and index finger on trackpad to zoom/rotate/pan the image.
        \item Find the image of [Animal].
        \item Zoom in on [Body Part] 
 of the [Animal].
        
    \end{enumerate} & 
    \begin{enumerate}[1. , leftmargin=*, nosep]
        \item Thumb, index finger, and middle finger can all be used for painting. Each finger can be bound with different brush style. Brush style will be displayed in the form of  cubes floating around fingertips.
        \item Tap on control panel to choose brush size and color for the touching finger.
        \item Choose [Color] with index finger.
        \item Draw [Object1] in the middle of the canvas.
        \item Choose [Color] with middle finger.
        \item Choose [Brush Size] with middle finger.
        \item Draw [Object2] with middle finger.
        \item Choose the eraser with thumb.
        \item Erase [Object1] or [Object2].
 
    \end{enumerate} & 
    \begin{enumerate}[1. , leftmargin=*, nosep]
        \item Type with index finger.
        \item Move the cursor by swiping middle finger leftwards/rightwards on keyboard.
        \item Enter "[Word1] [Word2]" in the input box.
        \item Move the cursor between two words.
        \item Delete "[Word1]".
        \item Enter "[Word3]" at the beginning of the line.
        
    \end{enumerate} \\
    \bottomrule
  \end{tabularx}
  \vspace{0.2cm}
\end{table*}
% \end{landscape}
